# Supplementary material for: Distributed Identification of Central Nodes with Less Communication
Source: arXiv:2106.14011 source file (2021-06-26)
Supplement: Supplementary file 1 [file appendix.tex]

\section*{Appendices}
\section{Communication failure} 
\label{sec:failure_detection}
So far we have introduced a pruning method for the problem of constructing a view of a communication graph, with an advantageous characteristic: pruning should reduce the number of messages exchanged between nodes during view construction. %Before quantifying the effect on the number of messages in Section \ref{sec:analysis}, we discuss how to handle communication failures for robustness. %A realistic robotics aspect is worth to be taken into account in pruning methods. 
Network communication is subject to failures: some nodes or edges could malfunction at any time. It is assumed that pruned nodes can not fail when building network views using our proposed pruning method. %A pruning method should treat the case of communication failures. In what follows we consider communication failure in pruning methods. 

This section considers communication as the exchange (sending and receiving) of messages or information between adjacent nodes in a network. We are restricted to peer-to-peer communication because nodes have limited communication capacity. Communication is successful when messages sent  are received uncorrupted, and ineffective communication is considered as a failure. There are two main techniques involved in communication failures to enable reliable delivery of messages which are: error detection and error correction. The former is the detection of malfunctions of some entities (nodes or edges) in the network. The latter not only detects errors, but also reconstructs the original message to produce an error-free message. In this paper, we consider error detection only, i.e. we can only detect failure of a functioning node/edge or recovery of a failed node/edge.  We consider a technique to detect and recover from communication failures when applying our pruning method. We next review some existing methods for failure detection and handling of recovery from communication failures.
%\paragraph{Failure model.}
%To fairly compare the amount of communication between our proposed pruning method and the benchmark method in case of failures we assume the following.
%Let $p_f$ and $p_r$ ($0<p_f<1$ and $0<p_r<1$) denote the probability that a node/edge  fails or recovers at  the end of each iteration respectively. It should be noted that each node/edge fails or recovers independently at the end of each iteration for both algorithms and these are conditional probabilities, i.e. these are the probability that a working node/edge fails, and the probability a failed node/edge recovers.  %At the end of each iteration of both algorithms, functioning nodes/edges independently fail with probability $p_f$. Similarly, failed nodes/edges independently recover from failures with probability $p_r$.
\subsection{Background of methods for failure detection}
There are several solutions for communication failures such as those described in \cite{pasin2008failure, kshirsagar2012survey}. Based on architectural organization, solutions to communication failures are grouped into two categories: centralized and decentralized approaches \cite{pasin2008failure}. Centralized solutions have a single node which detects and manages failures in the system. For example, \cite{stoller1997leader} proposed a simple centralized solution for failure detection: it proposes implementing a failure detector (FD)\label{communication:FD} to detect and report failures of nodes, and also to report the restoration  of nodes when they recover. When the FD detects the failure of a node, it reports a down signal to other nodes. Note that in \cite{stoller1997leader}, the FD is a separate module which monitors all the nodes. In this paper, we are interested in decentralized solutions.

%There are several decentralized solutions for dealing with communication failures.  
\cite{kshirsagar2012survey} grouped decentralized solutions for management of communication failures into three categories: 
\begin{itemize}
	\item node self-detection approaches, where  each node  can  identify its own malfunction   by   performing  self-diagnosis;
	\item neighbour coordination approaches, where nodes coordinate  with  their immediate neighbours  to  detect malfunctioning nodes and report their recoveries; and
	\item  clustering approaches, where the entire network is split into clusters and each cluster has a local coordinator responsible for performing tasks for failure   management task. %Here, heartbeat diffusion \cite{tai2004cluster} can be adopted to identify  failed nodes in each cluster. A heartbeat is a periodic signal to indicate desirable operation of a network system.
\end{itemize}

From the three categories of decentralized approaches for failure detection, we find the neighbour coordination approach proposed in \cite{sheth2005decentralized} most suitable. %suitable for our pruning methods simply because a node needs to know which of its neighbours have failed.
The disadvantage of the node self-detection approach is that a node is not aware of failure of other nodes in the system. This approach may be suitable for monitoring system where one needs to study, for example, the impact of failure of a node in the entire system without propagating such information to other components of the system. The clustering approach is quite similar to the neighbour coordination approach, but the former is inappropriate for our use since it requires that the network be split in advance and that the local coordinators be known to other cluster members. In the neighbour coordination approach, each node can monitor the behaviour of its immediate neighbours, which suits our decentralised approach well. 

%The selection or design of a suitable solution for communication failure depends on some assumptions such as the type of communication (e.g. synchronous or asynchronous). For our case, we find the neighbour coordination solution proposed in \cite{sheth2005decentralized} suitable. %to adapt in pruning algorithms because of its simplicity.  %Here we apply the FD differently. 
%In \cite{sheth2005decentralized}, the failure detection functionality is implemented in each node, as required by the decentralised nature of our problem. Thus each node is able to monitor other nodes in its neighbourhood.

As taken here, two situations can cause communication failure. First, a node can fail to send a message. Second, a communication channel (i.e. an edge) can fail to (fully) transmit a message. %It was mentioned earlier (Section \ref{sec:architecture}) that nodes have six states. The failure of a node adds another stage. 
A node or an edge is said to be down when it fails to transmit messages/information. For our purposes, a node will only need to know the states of nodes and edges in its neighbourhood.

We next describe the approach (Algorithm \ref{algo:pruning_fd}) we propose for failure detection.
\subsection{Neighbour coordination approach}
In our case, each node will have a FD component to monitor its immediate neighbours or incident edges in order to detect and report their failures. It also reports when failed nodes and edges recover. In other words, a node is monitored by all its immediate neighbours and an edge is monitored by both nodes that the edge connects. %Only one FD node can report failure and restoration of a node or edge to other nodes in the network. When some node fails, the node with the smallest identifier is considered to be the FD.
% how a failure is detected
There are two ways a node can detect failure of its neighbour or an incident edge. A node $v_i$ considers another node $v_j$ in its neighbourhood down if $v_i$ does not receive a message from $v_j$ for $T$ units of time (the variable $T$ is user-defined), unless the node $v_j$ is on hold. %Two nodes are neighbours when they are adjacent. 
It is assumed that any other nodes, say $v_k$, than the failed node $v_j$ assigns the same $T$ to $v_j$.
%But if a node does not receive a message from its neighbour after time $T$, this might not mean that the neighbour has failed. A big $T$ could also mean that some information are coming from a very long distance, due to the size of the network for instance. Such information may be ignored for the sake of coordination. 
We use checksums  in our various algorithms to detect failure in communication channels. In our algorithms, checksums is a boolean function: it returns false if no errors were detected during transmission, otherwise it returns true.  %The quantity $T$ is given as follows. 
%
%Let $n$ and $m$ be the width and the height of the search environment, $\gamma$ and $d$ be the velocity and communication range of a node, and $\tau$ be the search time. Let $N_m$ denote the maximum number of serendipitous interactions a node can be member of, and $T_{\Delta m}$ be expected interval between occurrence of two interactions with respect to a node. 
%Assuming sending of a message from a node to another node takes $t_u$ unit of time, a reasonable time $T_j$ a node $v_j$ should take to send messages to all its neighbours is
%\begin{equation}
%\label{eq:failure_time}
%T_j =t_u\,d_j\,,
%\end{equation}
% where $d_j$ denotes the degree of $v_j$. 
%We define the time $T_{ij}$ which a node $v_i$ uses to detect the failure of another node $v_j$ by 
%\begin{equation}
%\label{eq:failure_time}
%T_{ij}=\frac{4}{3}\, t_u\,d_j\,.
%\end{equation}
%Given a number of nodes in an interaction, it is clear that a path graph would be the worst topology of an ad-hoc network formed in the interaction of nodes, in terms of propagation of messages in the network. Assuming that the total number of nodes which can meet at a time is known, that should be $T$.

%On the other hand, detection of channel failure is not trivial. One way to detect failure of a channel which we consider here, when sending a message, a node sends also the size of the message along. An edge $(i, k)$ is put down if in the message received by $v_i$ we notice the following. Either the information about the size of message is missing or does not reflect the actual message received.

The value of $T$ depends on the maximum number of iterations. For a typical value of $D$, $T$ can be set to $1$ second for $D$ iterations corresponding to $D$ seconds (i.e. $1$ second corresponds to $1$ iteration), as done in our experiments. We choose $1$ second because each node is supposed to receive information from its neighbours at the end of each iteration (i.e. every second). This indicates that when a node does not send information for at least $T=1$ second, the node can be identified by its neighbours as failed.

To inform its immediate neighbours about the failure of a node or the failure of a channel, the node $v_i$ sends a down signal to its immediate neighbours. %In case of failure of node $v_j$ or edge $e_{ij}$, a FD node $v_i$ only reports to its neighbours which are not neighbours to $v_j$. 
Nodes relay these signals further through the network. This approach can lead to loops of failure signals. To avoid such loops, each signal is uniquely identified by the FD nodes. %\textemdash we assume that when a node (or an edge) fails, all its immediate neighbours (or both nodes that the edge connects) detect the failure reliably (i.e. all the corresponding FD nodes for a failed node/edge have exactly the same view on the failed node/edge). 
Every node  stores failure signals it has received, which it removes when it receives a recovery signal corresponding to that failure signal. In this way, a node relays a failure signal only if such signal is absent in its storage memory under the assumption that a node or an edge only fails once per iteration (this is checked using the subroutine \textsc{isPersistent} in Algorithm \ref{algo:pruning_fd}). This means that if a non-neighbour of a failed node receives multiple failure signals of that failed node, it will only relay the first failure signal. Also a node sends or relays a failure signal to a neighbour only after receiving a message from it. In this way, loop avoidance will be reinforced. The format of a failure signal is $\langle \texttt{Signal($S, Q, i, c$)}\rangle$ to denote a signal concerning $c$ ($c$ is either an edge or a node) of type $S$ and $Q$ ($S$ and $Q$ are used to indicate whether it is a failure signal or a recovery signal) is sent from the node $v_i$. For failure of a node $v_j$, the signal sent by $v_i$ is $\langle \texttt{Signal($0,0, i, j$)}\rangle$. For failure of an edge $e_{jk}$, the signal sent by $v_i$ is $\langle \texttt{Signal($0,1, i, e_{jk}$)}\rangle$.

If some node is down, other nodes keep exchanging messages. Whatever its condition (failed or not), an edge is always used by both the nodes incident to it. In other words, if an edge is down, both the nodes incident to it keep exchanging messages through the failed channel until a possible recovery of the failed edge (i.e. until a message is successfully received)\textemdash a better approach might be to poll the connection periodically, after increasing intervals. Otherwise, they will never know the recovery of the edge when that happens. If there is still some failed nodes or edges which have not recovered by the end of view construction, functioning nodes shall remove them from their final views (see Line \ref{removal} in Algorithm \ref{algo:pruning_fd}). %Two situations can arise in the case of node or edge failure. The two situations will be treated differently. 
%\begin{enumerate}
%	\item The first situation happens when the failed node is a cut node. Its failure will then give rise to multiple connected components.
%	\item  
A failed node or edge can speed up or delay the communication process between nodes. That is because the removal of a node or edge from a network can change path lengths between remaining nodes (Figure \ref{fig:removal}) and thus the complexity of the process of constructing a view. 

When a failed node or edge is restored, the FD nodes send a restoration signal to their immediate neighbours, for relaying through the network. A failed node is considered restored when the FD node receives a message from it. Also a failed edge is considered restored when it is successful. %Similarly to failure signals, recovery signals are also uniquely identified by the FD nodes to avoid loops of signals. 
For restoration of a node $v_j$, the signal sent by node $v_i$ is $\langle \texttt{Signal($1, 0, i, j$)}\rangle$. For restoration of an edge $e_{jk}$, the signal sent by node $v_i$ is $\langle \texttt{Signal($1, 1, i,e_{jk}$)}\rangle$.  A node that recovers should simply carry on sending neighbouring messages. A node stores failure signals in a queue $\mathcal{P}_i$. 

There are four situations for the report of failure. The first situation is when a node, say $v_i$, has detected a failure of a node in its neighbourhood. The second situation is when the node $v_i$ has detected a failure of an edge in its neighbourhood. The third situation is when the node $v_i$ has detected a recovery in its neighbourhood. The fourth situation is when a node $v_i$ has received a failure or recovery signal from its neighbour, which means the node $v_i$ is not a neighbour of the failed node or incident to the failed edge. In the last case, it can forward the signal received to its other neighbours. As mentioned before,  a node relays a failure signal if only such signal is absent in its storage memory (this is checked using the subroutine \textsc{isPersistent} in Algorithm \ref{algo:pruning_fd}).  The approaches for these four situations are given in Algorithm \ref{algo:pruning_fd} (see procedures \textsc{nodeFailureDetection}, \textsc{edgeFailureDetection}, \textsc{recoveryDetection} and \textsc{forwardFailureSignals}). %In  Algorithm \ref{algo:pruning_fd}, the set \label{pruning:upanddown} $\mathcal{N}^{down}_i$ denotes the set of failed nodes known by $v_i$; the set $\mathcal{S}^{down}_i$ denotes the set  of failed edges known by $v_i$; and the set $\mathcal{E}^{down}_i$ denotes the set of nodes in $\mathcal{N}_i$ incident to at least one edge in $\mathcal{S}_i^{down}$.

One might argue that a node which receives a neighbouring message from its neighbour which has just recovered from a failure needs to consider the time of failure of its neighbour while integrating the message received.  Otherwise, it may end up with an incorrect view of the communication network. This would have been true in the case where neighbouring information was described by nodes only, as one may need to know which nodes are direct neighbours for an effective integration. In our case, neighbouring information is represented by edges (i.e. from neighbouring information a node knows which nodes are direct neighbours), so there is no need to consider time of failure while a node is integrating the message received.
%When a node receives neighbouring message $\langle NeighbouringMessage(S_j^t)\rangle$ from another which has just recovered from a failure, it needs to consider when the node failed while integrating the message received. Otherwise, it may end up with an incorrect view of the communication network.% as messages sent by the recovered node may have some shift. 

\begin{figure}[h]
	\centering
	\begin{subfigure}{0.15\textwidth}
		\includegraphics[width=\textwidth]{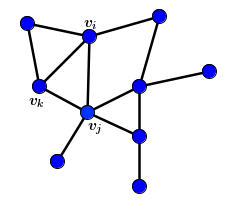}
		\caption{}
		\label{fig:removal_init}
	\end{subfigure}
	\begin{subfigure}[h]{0.15\textwidth}
		\includegraphics[width=\textwidth]{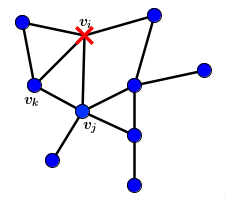}
		\caption{}
		\label{fig:removal_node}
	\end{subfigure}
	\begin{subfigure}[h]{0.15\textwidth}
		\includegraphics[width=\textwidth]{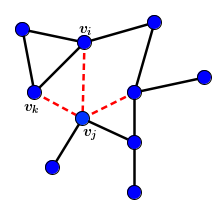}
		\caption{}
		\label{fig:removal_edge}
	\end{subfigure}	
	\caption[\textit{Illustration of failure of a node or edges.}]{\textit{\small{Illustration of failure of a node or edges. \textbf{(\ref{fig:removal_init})}: Initial configuration of a communication graph with a diameter of $4$.
				\textbf{(\ref{fig:removal_node})}: Failure of the node $v_i$ to communicate. The new graph has a diameter of $4$. \textbf{(\ref{fig:removal_edge})}: Failure of the three edges in dashed red lines. The new graph has a diameter of $6$.}}}
	\label{fig:removal}
\end{figure}
%\begin{figure}
%	\centering
%	\begin{subfigure}[h]{0.45\textwidth}
%		\includegraphics[width=\textwidth]{figs/leader/rearrangement.png}
%		\caption{}
%		\label{fig:rearrangementinit}
%	\end{subfigure}
%	\begin{subfigure}[h]{0.45\textwidth}
%		\includegraphics[width=\textwidth]{figs/leader/rearrangement1.png}
%		\caption{}
%		\label{fig:rearrangement1}
%	\end{subfigure}
%	\begin{subfigure}[h]{0.45\textwidth}
%		\includegraphics[width=\textwidth]{figs/leader/rearrangement2.png}
%		\caption{}
%		\label{fig:rearrangement2}
%	\end{subfigure}	
%	\caption[\textit{Illustration of re-arrangement of a network after the failure of a cut node. }]{\textit{\small{Illustration of re-arrangement of a network after the failure of a cut node. \textbf{(\ref{fig:rearrangementinit})}: Initial configuration of a communication graph.
%				\textbf{(\ref{fig:rearrangement1})}: Failure of the cut node $v_j$ which generates two connected components. \textbf{(\ref{fig:rearrangement2})}: Re-arrangement of the node $v_l$ to reconnect the network. The node $v_l$ has moved to a new position and the dashed red line is a new edge that reconnects the network.}}}
%	\label{fig:rearrangement}
%\end{figure}

\begin{algorithm}
	%\hspace*{\algorithmicindent} \textbf{Input:} $D$\\
	%\hspace*{\algorithmicindent} \textbf{Output:} $\mathcal{S}_{t, i}$
	\begin{algorithmic}[1]
		\scriptsize
		\Procedure{runPruningFD()}{}
		\State \texttt{PruningobjectFD}$\gets$\textsc{pruningWithFD}($\mathcal{N}_i, D, T$)
		\State \texttt{PruningobjectFD}.\textsc{initialOneHop()}
		\State \texttt{PruningobjectFD}.\textsc{initialUdate()}
		\State \texttt{PruningobjectFD}.\textsc{firstPruningDetection()}
		\While{\NOT \texttt{PruningobjectFD}.\textsc{isEnded()}}
		\State \texttt{PruningobjectFD}.\textsc{nextOneHop()}
		\State \texttt{PruningobjectFD}.\textsc{nextUpdate()}
		\EndWhile
		\State \texttt{PruningobjectFD}.\textsc{finalIteration()}
		\EndProcedure
		\State
		\Class{pruningWithFD}
		\State \textbf{\underline{Class variables}}
		\State  \makebox[2cm][l]{$A$} set of current neighbours of $v_i$
		
		\State  \makebox[2cm][l]{$\Gamma_i$} the set of signals received by $v_i$
		\State \makebox[2cm][l]{$\mathcal{E}^\mathrm{down}_i$} the set of nodes in $\mathcal{N}_i$ incident to at least one edge in  $\mathcal{S}_i^\mathrm{down}$
		
		\State \makebox[2cm][l]{$\mathcal{N}^\mathrm{down}_i$} set of failed nodes known by $v_i$ 
		\State \makebox[2cm][l]{$\mathcal{N}_{i, t}^\mathrm{up}$} set of neighbours of $v_i$ which are still involved in interaction at iteration $t$
		\State \makebox[2cm][l]{$\mathcal{P}_{i}$} the queue of failure signals received  by node $v_i$
		\State \makebox[2cm][l]{$\mathcal{S}^\mathrm{down}_i$} set  of failed edges known by $v_i$

		%\State \makebox[2cm][l]{$t_j$} time of failure;
		\State \makebox[2cm][l]{$T$} maximum number of iterations for a node to detect failures of its neighbours 
		\State \makebox[2cm][l]{$T_{ij}$} the last time node $v_i$ received a message from node $v_j$ 
		
		\\\hrulefill
		\Constructor{$\mathcal{N}_i, D, T$}
		\State $(\mathcal{N}_i, D, T)\gets (\mathcal{N}_i, D, T)$
		\State $(\Gamma_i, \mathcal{N}^\mathrm{up}_{i, t},\mathcal{S}^{(0)}_i) \gets (\emptyset, \mathcal{N}_i.\texttt{clone()}, \{e_{ij}: \forall v_j\in\mathcal{N}_i \})$
		%\State $\mathcal{S}^{(0)}_i\gets  \{e_{ij}: \forall v_j\in\mathcal{N}_i \}$
		%	\State $\mathcal{N}^\mathrm{up}_{i, t} \gets \mathcal{N}_i$\label{line:pruning_endfd}
		%\State $A\gets \mathcal{N}_i$
		\State $\mathcal{S}_{i, 0}\gets \mathcal{S}^{(0)}_i$.\texttt{clone()} \Comment{``$v_i$ detects its immediate neighbours''}\label{line:initiation_endfd} 
		\State   $(\mathcal{N}_i^\mathrm{down}, \mathcal{S}_i^\mathrm{down}, \mathcal{E}^\mathrm{down}_i, \mathcal{S}^{(1)}_i) \gets (\emptyset,\emptyset,\emptyset,\emptyset)$
		\EndConstructor
		\State
		\Procedure{nextOneHop()}{}
		\If{\NOT \textsc{isEnded()}}
		\State $t\gets t+1$
		\State $\mathcal{N}^\mathrm{up}_{i, t}\gets \mathcal{N}_{i}\setminus (\mathcal{F}_{i, t}\cup \mathcal{N}_i^\mathrm{down} \cup \mathcal{E}^\mathrm{down}_i)$
		\State  $\mathcal{S}^{(t)}_i\gets \emptyset$
		%\STATE 
		%\STATE \texttt{failureBroadcasting2($v_j$)}
		\For{$v_j \in \mathcal{N}^\mathrm{up}_{i, t}$}
		\State $v_i$ sends $\langle \texttt{NeighbouringMessage($i, \mathcal{S}_i^{(t-1)}$)}\rangle$
		to $v_j$
		%\STATE \texttt{failureBroadcasting1()}
		%\STATE \texttt{failureBroadcasting2()}
		
		\EndFor
		\EndIf
		\EndProcedure
		\State
		\Procedure{nextUpdate()}{}
		\If{\NOT \textsc{isEnded()}}
		
		%\State $A\gets \mathcal{N}^{up}_{i,t}$
		%\While{$A\neq \emptyset$}
		\While{$\mathcal{M}_i.\texttt{size()}\geq 1$}

		\For{$v_k\in \mathcal{N}^{up}_{i,t}$}
		\State \textsc{nodeFailureDetection($v_k$)}
		\EndFor
		%\If { $v_i$ receives $\langle \texttt{NeighbouringMessage($\mathcal{S}_j^{(t-1)}$)}\rangle$ from $v_j$}
		\State $(j,\mathcal{S}_j^{(t-1)}) \gets \mathcal{M}_i.\texttt{dequeue}()$
		\State $T_{ij}\gets$\texttt{currentTime()}
		\State \texttt{isDown}$\gets$\textsc{edgeFailureDetection($S_j^{(0)}$)}
		%\State \texttt{hasFailed}$\gets $\texttt{checksums($S_j^{(t-1)}$)}

		\algstore{pruningwithFD}
	\end{algorithmic}  
	\caption[\textit{Our proposed pruning method with failure management.}]{\textit{Our proposed pruning method with failure management. The algorithm gives the code executed for node $v_i$. We use a class concept to implement this benchmark method and the class is initialised by a constructor (see \textbf{constructor}).} \textit{ The main methods are  \textsc{nextOneHop} and \textsc{nextUpdate} which are run by $v_i$ once each iteration.  Apart from the variables used in Algorithm \ref{algo:pruning}, additional global variables of this algorithm  are listed in the beginning of the algorithm.
			It should be noted that in this algorithm assignments make copies of objects. An example of code to execute the class is given in the procedure \textsc{runPruningFD}.}}
	\label{algo:pruning_fd}
\end{algorithm}

\begin{algorithm}
	\begin{algorithmic}[1]
		\scriptsize
		\algrestore{pruningwithFD}
		\If{!\texttt{isDown}}
		\State $\mathcal{S}^{(t)}_i\gets \mathcal{S}^{(t)}_i \cup \mathcal{S}^{(t-1)}_j$ 
		\Comment{``$v_i$ fuses the messages received''}
		%\STATE $\mathcal{S}^{t}_i\gets \mathcal{S}^{t}_i \cup \mathcal{S}^{t-1}_j$ \COMMENT{"subsequent receptions of messages"}
		%\State \textsc{recoveryDetection($v_j$)}
		%\State \textsc{forwardFailureSignals($v_j$)}
		%\State $A\gets A\setminus\{v_j\}$
		\EndIf
		\State \textsc{recoveryDetection($v_j$}, \texttt{isDown})
		%\State \textsc{edgeFailureDetection($v_j$}, \texttt{hasFailed})
		%\State $\mathcal{M}_i.\texttt{dequeue}(0)$
		%\EndIf
		
		%\If { $v_i$ suspects a failure between it and a neighbour $v_j$}
		%\STATE $\mathcal{S}^{t}_i\gets \mathcal{S}^{t}_i \cup \mathcal{S}^{t-1}_j$ \COMMENT{"subsequent receptions of messages"}
		%\State $A\gets A\setminus \{v_j\}$
		
		%\EndIf
		
		\State $\mathcal{N}^\mathrm{up}_{i, t}\gets \mathcal{N}^\mathrm{up}_{i, t}\setminus (\mathcal{N}_i^\mathrm{down} \cup \mathcal{E}^\mathrm{down}_i)$
		
		%\EndFor
		\EndWhile
		\State \textsc{forwardFailureSignals()}
		\State $\mathcal{S}^{(t)}_i\gets \mathcal{S}^{(t)}_i\setminus \mathcal{S}_{t-1, i}$ 
		\State $\mathcal{S}_{t, i}\gets \mathcal{S}_{t-1, i}\cup \mathcal{S}^{(t)}_i$
		%\IF{\texttt{repetition}$==$\texttt{True}}
		%\STATE $\mathcal{F}^{(t)}_i\gets \emptyset$
		\State $\mathcal{F}^{(t)}_i\gets$ \textsc{furtherPruningDetection()} \Comment{``$v_i$ detects elements of $\mathcal{F}^{(t)}_i$ in its neighbourhood, defined in Algorithm \ref{algo:pruning}''}
		%\STATE $\mathcal{F}_i\gets \mathcal{F}_i\cup \mathcal{F}_i^{(t)}$
		\State $\mathcal{F}_{i, t}\gets \mathcal{F}_{i, t} \cup \mathcal{F}^{(t)}_{i}$
		\EndIf
		\EndProcedure
		\State
		\Procedure{initialOneHop()}{}
		\State $t\gets 1$
		\For{$v_j \in \mathcal{N}_i$}
		\State $v_i$ sends $\langle \texttt{NeighbouringMessage($i, \mathcal{S}_i^{(0)}$)}\rangle$
		to $v_j$
		\State $T_{ij}\gets$\texttt{currentTime()}
		\EndFor
		\EndProcedure
		\State
		\Procedure{initialUpdate()}{}
		
		\While{$\mathcal{M}_i.\texttt{size()}\geq 1$}
		\For{$v_k \in \mathcal{N}_{i, t}^{\mathrm{up}}$}
		\State \textsc{nodeFailureDetection($v_k$)}
		\EndFor
		\State $(j, \mathcal{S}_j^{(0)}) \gets \mathcal{M}_i.\texttt{dequeue}()$

		%\If {$v_j\in A$ \AND $v_i$ receives $\langle \texttt{NeighbouringMessage($\mathcal{S}_j^{(0)}$)}\rangle$}
		\State $T_{ij}\gets$\texttt{currentTime()}
		%\State %\texttt{failure}$\gets$\texttt{checksums($S_j^{(0)}$)}
		\State \texttt{isDown}$\gets$\textsc{edgeFailureDetection($S_j^{(0)}$)}\Comment{``it returns false if no error was detected.''}
		\If{!\texttt{isDown}}
		\State $\mathcal{S}^{(1)}_i\gets \mathcal{S}^{(1)}_i \cup \mathcal{S}^{(0)}_j$
		\Comment{``$v_i$ fuses the messages received''}	
		\State $\mathcal{Q}_{ij}\gets \mathcal{S}^{(0)}_{j}$.\texttt{clone()}
		
		%	\State \textsc{forwardFailureSignals($v_j$)}
		%\State $A\gets A\setminus\{v_j\}$
		\EndIf
		\State \textsc{recoveryDetection($v_j$}, \texttt{isDown})
		%\State \textsc{edgeFailureDetection($v_j$}, \texttt{hasFailed})
		%\EndIf
		%\State $\mathcal{M}_i.\texttt{dequeue}(0)$
		%\EndFor
		\State $\mathcal{N}^\mathrm{up}_{i, t}\gets \mathcal{N}^\mathrm{up}_{i, t}\setminus (\mathcal{N}_i^\mathrm{down} \cup \mathcal{E}^\mathrm{down}_i)$
		\EndWhile
		\State \textsc{forwardFailureSignals()}
		
		\State $\mathcal{S}^{(1)}_i\gets \mathcal{S}^{(1)}_i\setminus \mathcal{S}_{i, 0}$ 
		\State $\mathcal{S}_{i, 1}\gets \mathcal{S}_{i, 0}\cup \mathcal{S}^{(t)}_i$\label{line:first_iteration_endfd}
		%\STATE $ r\gets 0$ 
		%\STATE $\mathcal{F}^{(t)}_i\gets \emptyset$
		
		\State  \textsc{firstPruningDetection()} \Comment{``$v_i$ detects leaves in its neighbourhood using Algorithm \ref{algo:pruning}''}
		%\State $v_i$ removes nodes in $\mathcal{N}^\mathrm{down}_i$ and edges in $\mathcal{S}^\mathrm{down}_i$ from $\mathcal{S}_{i, t}$
		\label{line:free3} 
		
		%\STATE $\mathcal{S}^0_i\gets \emptyset$\label{line:initialisation_begin}
		\EndProcedure
		\State
		\Procedure{nodeFailureDetection}{$v_j$}\Comment{``a procedure to send a failure signal when a node detects failure of a neighbour in its neighbourhood''}
		\If{$\texttt{currentTime()}-T_{ij}>T$}
		\State $\mathcal{N}_{i, t}^\mathrm{up} \gets \mathcal{N}_{i, t}^\mathrm{up}\setminus \{v_j\}$
		%\STATE $\mathcal{N}_i^{up} \gets \mathcal{N}_i^{up}\setminus \{v_j\}$ \OR $\mathcal{S}_i^{up} \gets \mathcal{S}_i^{up}\setminus \{(\min(i, j), \max(i, j))\}$ 
		\State $\mathcal{N}_i^\mathrm{down} \gets \mathcal{N}_i^\mathrm{down}\cup \{v_j\}$
		%\STATE $v_i$ adds its neighbours which are incident to at least one edge in $\mathcal{S}_i^{down}$ to $\mathcal{E}^{down}_i$

		%\State \Return $\mathcal{S}_{i, t}, \mathcal{F}_{ i, t}$\label{line:end_pruningfd}
		\State $v_i$ sends $\langle \texttt{Signal($0, 0, i,j$)}\rangle$ to $\mathcal{N}^\mathrm{up}_{i, t}$	
		%\State $A\gets A\setminus \{v_j\}$
		\EndIf
		
		\EndProcedure
		\State
		\Function{edgeFailureDetection}{$v_j, \mathcal{S}_i^{(t)}$}\Comment{``a procedure to send a failure signal when a node detects failure of an edge in its neighbourhood''}
		\State $\texttt{isDown}\gets \texttt{checksum}(\mathcal{S}_i^{(t)})$
		\If{\texttt{isDown}}
		%\STATE $\mathcal{N}_{i}^{up} \gets \mathcal{N}_{i}^{up}\setminus \{v_j\}$
		%\STATE $\mathcal{N}_i^{up} \gets \mathcal{N}_i^{up}\setminus \{v_j\}$ \OR $\mathcal{S}_i^{up} \gets \mathcal{S}_i^{up}\setminus \{(\min(i, j), \max(i, j))\}$ 
		\State  $\mathcal{S}_i^\mathrm{down} \gets \mathcal{S}_i^\mathrm{down}\cup \{e_{ij}\}$
		\State $\mathcal{E}^\mathrm{down}_i\gets \mathcal{E}^\mathrm{down}_i\cup\{v_j\}$ %adds its neighbours which are incident to at least one edge in $\mathcal{S}_i^\mathrm{down}$ to $\mathcal{E}^\mathrm{down}_i$
		\State $v_i$ sends $\langle \texttt{Signal($0, 1,i,e_{ij}$)}\rangle$ to $\mathcal{N}^\mathrm{up}_{i, t}$	
		%\State $A\gets A\setminus \{v_j\}$
		\EndIf
		\State \Return $\texttt{isDown}$
		\EndFunction
		%\State

		\algstore{jordan}

	\end{algorithmic}  
\end{algorithm}
\begin{algorithm}  
	\begin{algorithmic}
		\scriptsize
		\algrestore{jordan}	
		\Procedure{recoveryDetection}{$v_j, \texttt{hasFailed}$}\Comment{``a procedure to send a recovery signal when a node detects recovery in its neighbourhood''}
		\If{$v_j \in \mathcal{N}_i^\mathrm{down}$}
		%\State %\texttt{failure}$\gets$\texttt{checksums($S_j^{(t)}$)}
		\If{!\texttt{hasFailed}}
		\State $\mathcal{N}_{i}^\mathrm{up} \gets \mathcal{N}_{i}^\mathrm{up}\cup \{v_j\}$
		%\STATE $\mathcal{N}_i^{up} \gets \mathcal{N}_i^{up}\cup \{v_j\}$ \OR $\mathcal{S}_i^{up} \gets \mathcal{S}_i^{up}\cup \{(\min(i, j), \max(i, j))\}$ 
		\State $\mathcal{N}_i^\mathrm{down} \gets \mathcal{N}^\mathrm{down}_i\setminus \{v_j\}$
		%\STATE $v_i$ removes its neighbours which are incident to at least one edge in $\mathcal{S}_i^{down}$ from $\mathcal{E}^{down}_i$
		\State $v_i$ sends $\langle \texttt{Signal($1, 0,i,j$)}\rangle$ to $\mathcal{N}^\mathrm{up}_{i, t}$
		\EndIf
		\EndIf
		\If{edge $e_{ij}\in \mathcal{S}_i^\mathrm{down}$}
		%\State %\texttt{failure}$\gets$\texttt{checksums($S_j^{(t)}$)}
		\If{!\texttt{hasFailed}}
		%\STATE $\mathcal{N}_{i}^{up} \gets \mathcal{N}_{i}^{up}\cup \{v_j\}$
		%\STATE $\mathcal{N}_i^{up} \gets \mathcal{N}_i^{up}\cup \{v_j\}$ \OR $\mathcal{S}_i^{up} \gets \mathcal{S}_i^{up}\cup \{(\min(i, j), \max(i, j))\}$ 
		\State  $\mathcal{S}_i^\mathrm{down} \gets \mathcal{S}_i^\mathrm{down}\setminus \{e_{ij}\}$
		\State $\mathcal{E}^\mathrm{down}_i\gets \mathcal{E}^\mathrm{down}_i\setminus\{v_j\}$
		\State $v_i$ sends $\langle \texttt{Signal($1, 1, i, e_{ij}$)}\rangle$ to $\mathcal{N}^\mathrm{up}_{i, t}$
		\EndIf
		\EndIf
		\EndProcedure
		\State
		\Function{isPersistent}{$\langle\texttt{Signal($S, Q,k, c$)}\rangle, \Gamma$}\Comment{``a procedure to check whether the node receives the signal for the first time''}
		\If{$\langle\texttt{Signal($S, Q,k, c$)}\rangle\not\in \Gamma$}
		\State $\Gamma \gets \Gamma \cup \{\langle\texttt{Signal($S, Q,k, c$)}\rangle\}$ 
		\State $\Gamma \gets \Gamma \setminus \{\langle\texttt{Signal($\neg S, Q,k, c$)}\rangle\}$ %\Comment{``if \texttt{Signal($SQ,k, c$)} is \texttt{Signal($00,k, c$)} then $\neg$\texttt{Signal($SQ,k, c$)} is \texttt{Signal($10, k, c$)} and vice-versa.''}
		\State \Return \TRUE
		\EndIf
		\State \Return \FALSE
		\EndFunction
		\State
		\Procedure{forwardFailureSignals()}{}\Comment{``a procedure to send a failure signal when a node receives a failure signal''}
		\While{$\mathcal{P}_i.\texttt{size()}\geq 1$}
		\State $(S, Q, k, c)\gets \mathcal{P}_i.\texttt{dequeue}()$
		%\If{$v_i$ has received $\langle \texttt{DownSignal($k$)}\rangle$ from its neighbour $v_j$}
		\If{\textsc{isPersistent}($\langle \texttt{Signal($S, Q,k,c$)}\rangle, \Gamma_i$) }
		\If{$S= 0 \AND Q=0$}
		\State $\mathcal{N}_i^\mathrm{down} \gets \mathcal{N}^\mathrm{down}_i\cup \{v_c\}$ 
		%\STATE $\mathcal{N}_i^{up} \gets \mathcal{N}_i^{up}\setminus \{v_k\}$ \OR $\mathcal{S}_i^{up} \gets \mathcal{S}_i^{up}\setminus \{(\min(k, l), \max(k, l))\}$
		\ElsIf{$S=0\AND Q=1$}
		\State  $\mathcal{S}_i^\mathrm{down} \gets \mathcal{S}_i^\mathrm{down}\cup \{c\}$
		\ElsIf{$S=1\AND Q=0$}
		\State $\mathcal{N}_i^\mathrm{down} \gets \mathcal{N}_i^\mathrm{down}\setminus \{v_c\}$
		\ElsIf{$S=1 \AND Q=1$}
		\State  $\mathcal{S}_i^\mathrm{down} \gets \mathcal{S}_i^\mathrm{down}\setminus \{c\}$
		\EndIf
		
		\State $v_i$ sends $\langle \texttt{Signal($S, Q,k,c$)}\rangle$ to $\mathcal{N}^\mathrm{up}_{i, t}$
		
		\EndIf
		%\If{$v_i$ has received $\langle \texttt{UpSignal($e_{kl}$)}\rangle$ from its neighbour $v_j$}
		%\If{\textsc{isPersistent}($\langle \texttt{UpSignal($e_{kl}$)}\rangle, \Gamma_i$) \AND !\texttt{checksums($\langle \texttt{UpSignal($e_{kl}$)}\rangle, \Gamma_i$)}}
		%\STATE $\mathcal{N}^{up}_i \gets \mathcal{N}^{up}_i\setminus \{v_k\}$ \OR $\mathcal{S}^{up}_i \gets \mathcal{S}^{up}_i\setminus \{(\min(k, l), \max(k, l))\}$
		%\State  $\mathcal{S}_i^\mathrm{down} \gets \mathcal{S}_i^\mathrm{down}\setminus \{e_{kl}\}$
		%\State $v_i$ sends $\langle \texttt{UpSignal($e_{kl}$)}\rangle$ to $\mathcal{N}^\mathrm{up}_{i, t}$
		%\EndIf
		%\EndIf	
		%\State $\mathcal{P}_i.\texttt{dequeue}(0)$
		\EndWhile
		\EndProcedure
		
		\State
		\Procedure{finalIteration()}{}
		
		\If{$t<D$}
		\For{$v_j \in \mathcal{N}^\mathrm{up}_{i, t}$}
		\State $v_i$ sends $\langle \texttt{NeighbouringMessage($i,\emptyset$)}\rangle$
		to $v_j$
		
		\EndFor
		\EndIf
		%\STATE $T \gets t$
		\State $\mathcal{S}_{i, t}\gets \mathcal{S}_{i, t}\setminus (\mathcal{S}^\mathrm{down}_i \cup \{e_{jk} \in \mathcal{S}_{i, t}: v_j \in \mathcal{N}^\mathrm{down}_i\lor v_k \in \mathcal{N}^\mathrm{down}_i \})$\label{removal}
		\EndProcedure
		\EndClass
	\end{algorithmic}  
\end{algorithm}

Our last step is to include the FD in the pruning method in Algorithm \ref{algo:pruning}. The new pruning algorithm including FD is presented in Algorithm \ref{algo:pruning_fd}. The main difference is that Algorithm \ref{algo:pruning_fd} takes into account detection and reporting of failures (and recovery).

The downside of this view construction approach with FD (Algorithm \ref{algo:pruning_fd}) is that there might be ambiguous situations where a node $v_i$ can wrongly think that it has reached an equilibrium state at the end of iteration $t$ because its $\mathcal{S}_i^{(t)}$ is found to be empty. This may arise in situations where there is an overload of failures. Such ambiguous situations are acceptable in this work because, as was motivated throughout this part, we do not expect network views across nodes to be the same or exact\textemdash each node considers the view it has constructed until the end of the procedure. It should also be noted that this approach invalidates the invariant that nodes know all their $t$-hop neighbours (in the underlying failure-free communication graph) after $t-1$ iterations.
